# Supplementary material for: Bayesian Models of Data Streams with Hierarchical Power Priors
Source: arXiv:1707.02293 source file (2017-07-07)
Supplement: Supplementary file 2 [file appendix.tex]

\appendix 
\newpage

\section{Proof of Theorems}

\section{Experimental Evaluation}

\subsection{Artificial Data}

\begin{figure}[htb!]
\vskip 0.2in
\begin{center}
\begin{tabular}{ccc}
\includegraphics[scale=0.3]{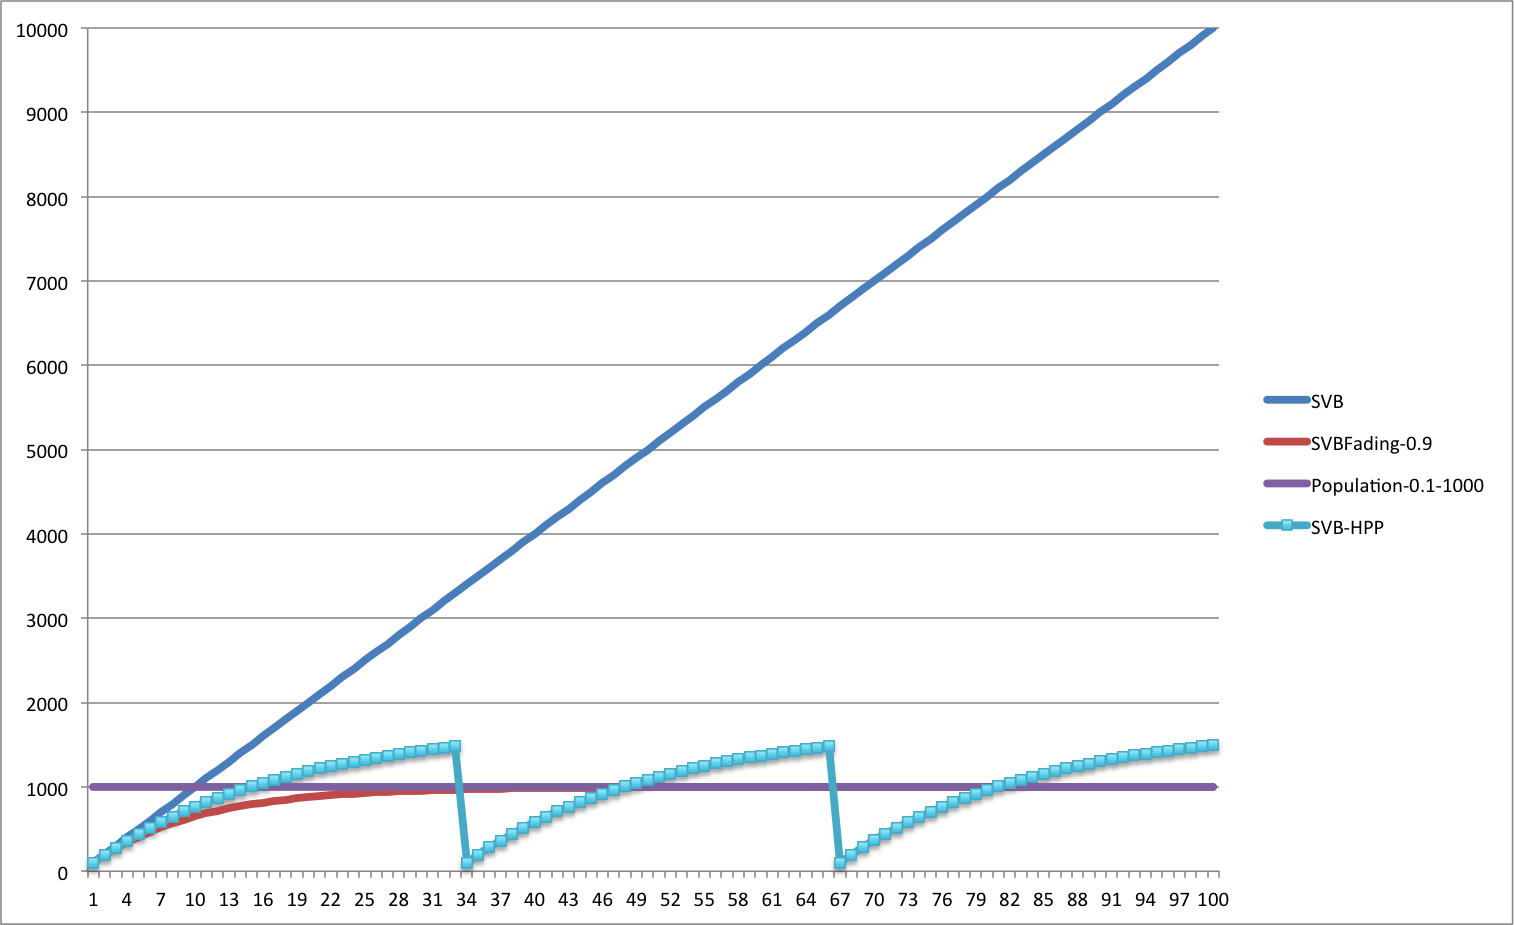}
\end{tabular}
\caption{$ESS_t$ for the Artificial Data Set with a Norma with fixed variance model}
\label{app:fig:exp:artificialESS}
\end{center}
\vskip -0.2in
\end{figure}

\begin{figure*}[htb!]
\vskip 0.2in
\begin{center}
\begin{tabular}{cc}
\includegraphics[scale=0.3]{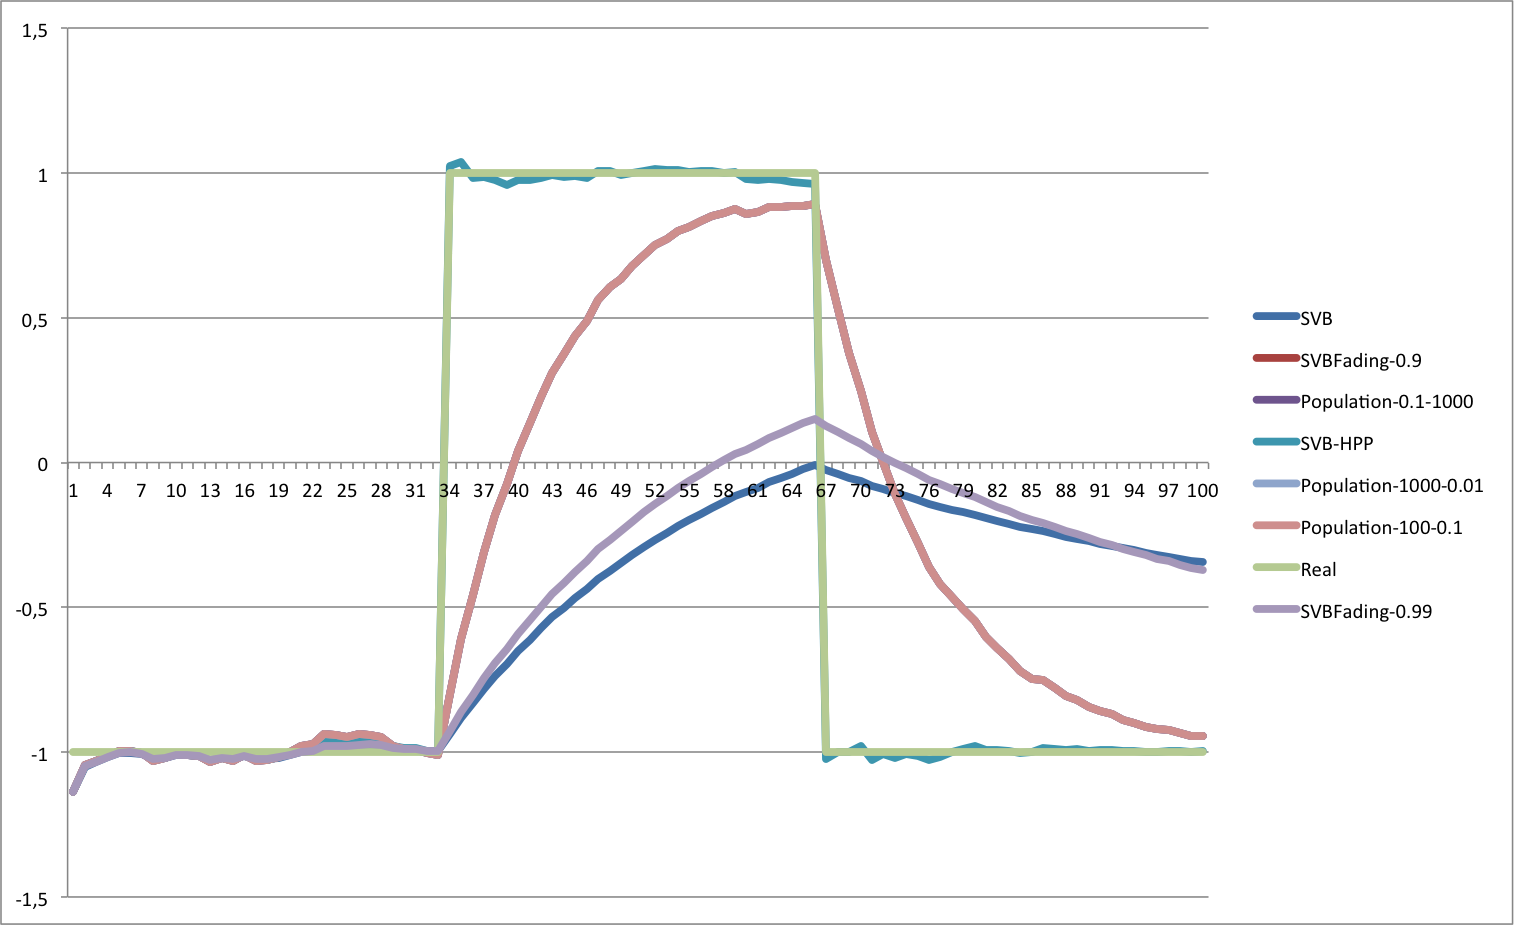}&
\includegraphics[scale=0.3]{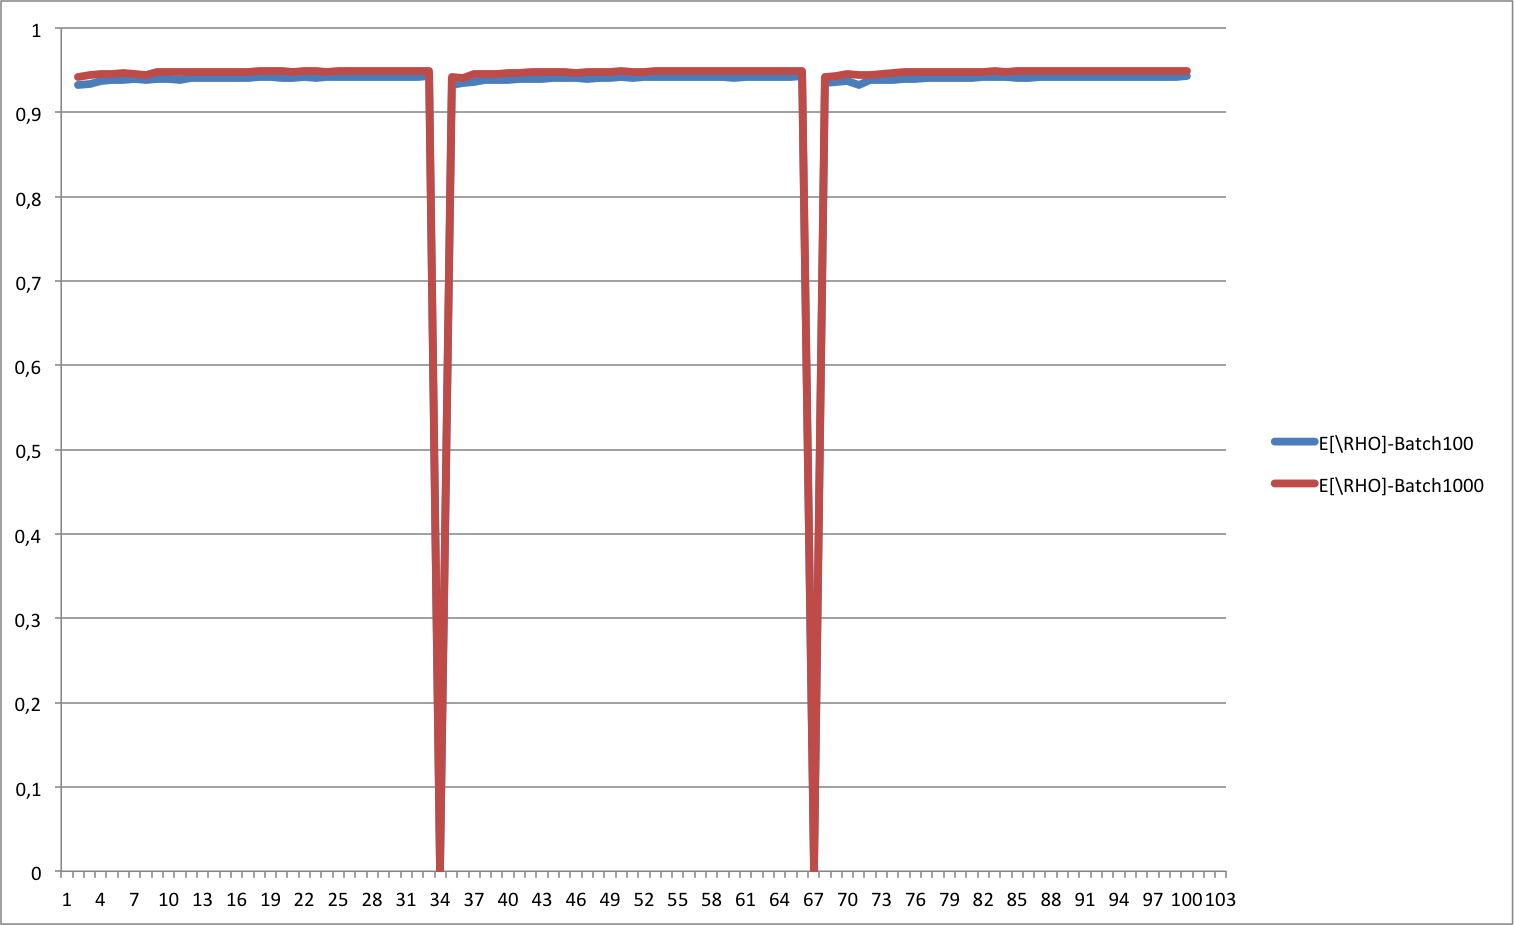}\\
(a) $E[\beta_t]$ & (b) $E[\rho_t]$ \\
\end{tabular}
\caption{Artifical Data Set-Normal with fixed Variance Model}
\label{app:fig:exp:artificialParemeter}
\end{center}
\vskip -0.2in
\end{figure*} 

\subsection{Real Life Data Sets}

\begin{figure*}[htb!]
\vskip 0.2in
\begin{center}
\includegraphics[width=8cm,height=4.5cm,keepaspectratio]{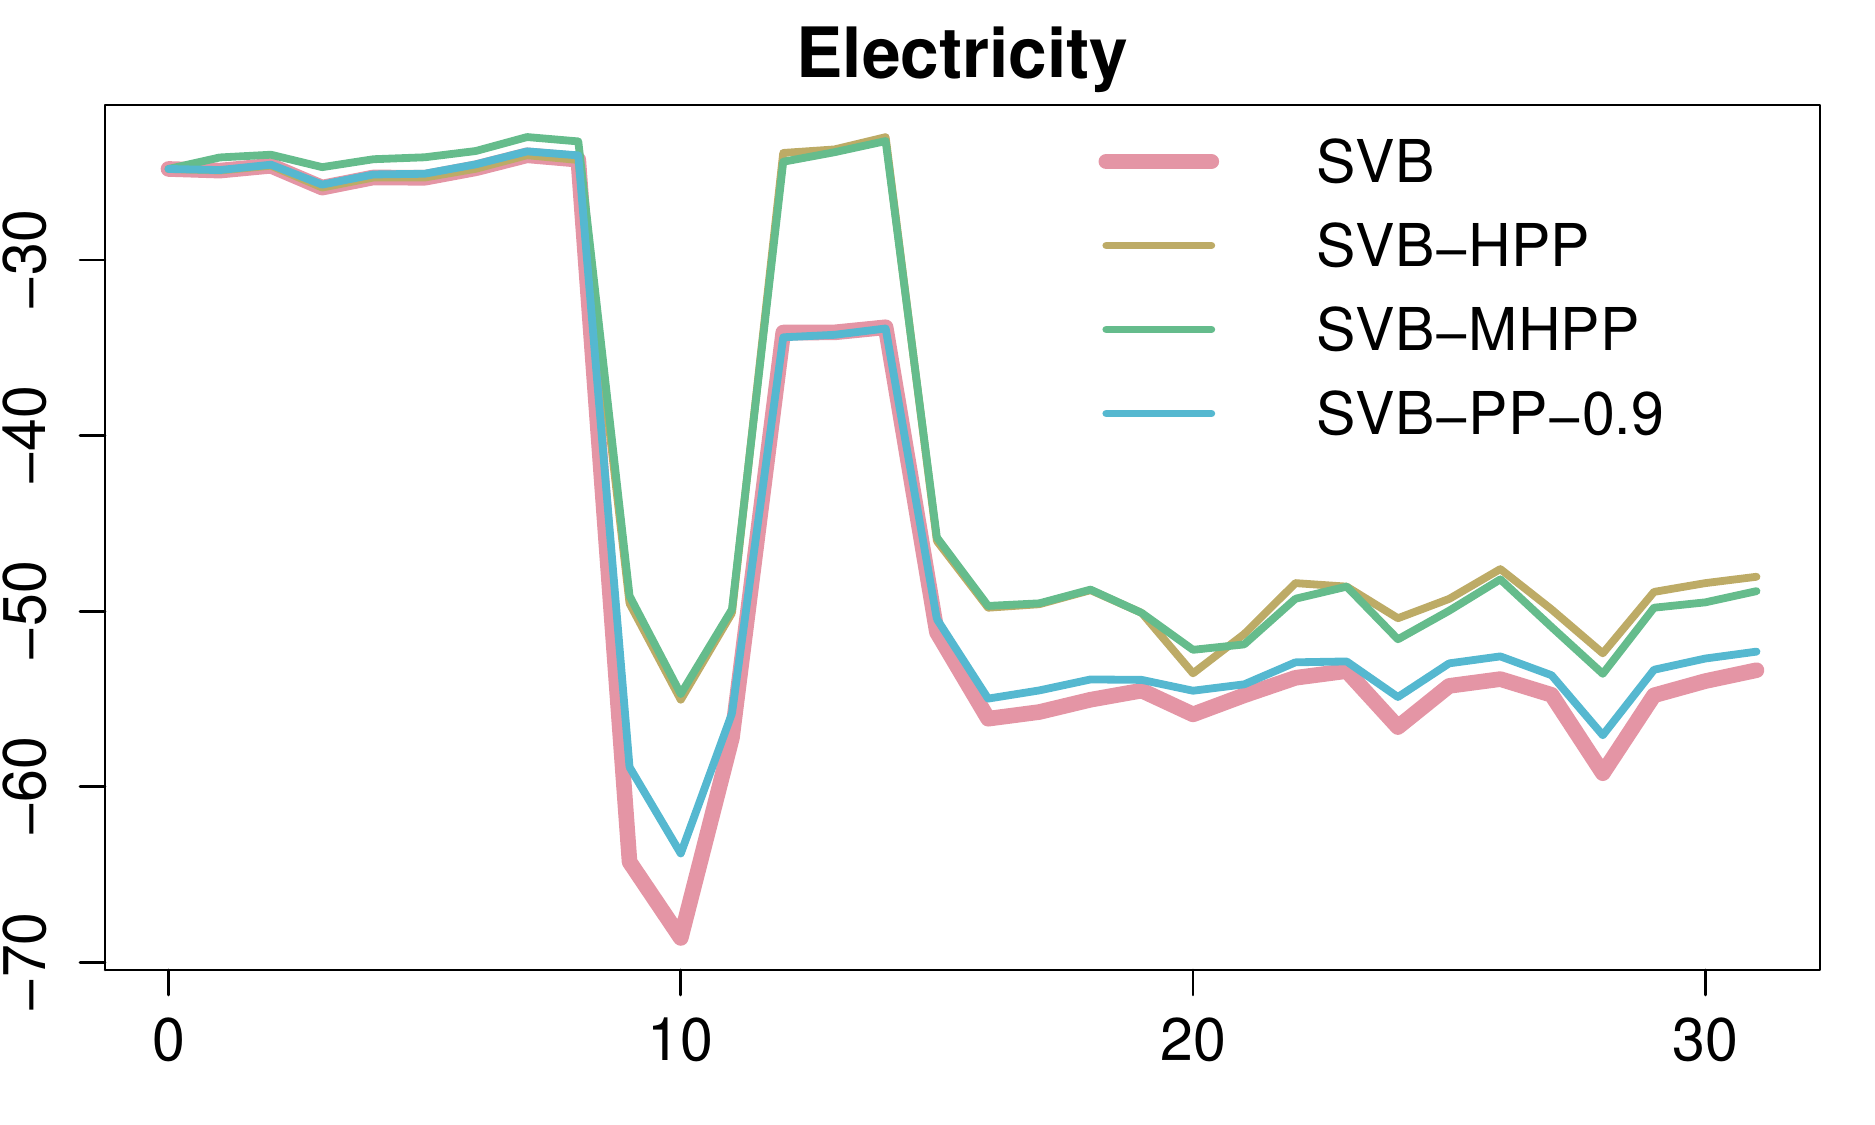}
%\begin{tabular}{cc}
%\includegraphics[scale=0.3]{figs/ELECTRICITY-TestMLL}&
%%\includegraphics[scale=0.2]{figs/ELECTRICITY-TotalMLL}&
%\includegraphics[scale=0.3]{figs/ELECTRICITY-RHO}\\
%(a) $TMLL_t$ & (b) $E[\rho_t]$ \\
%\end{tabular}
\caption{Electricity}
\label{app:fig:exp:elec}
\end{center}
\vskip -0.2in
\end{figure*}

\begin{figure*}[htb!]
\vskip 0.2in
\begin{center}
	\includegraphics[width=8cm,height=4.5cm,keepaspectratio]{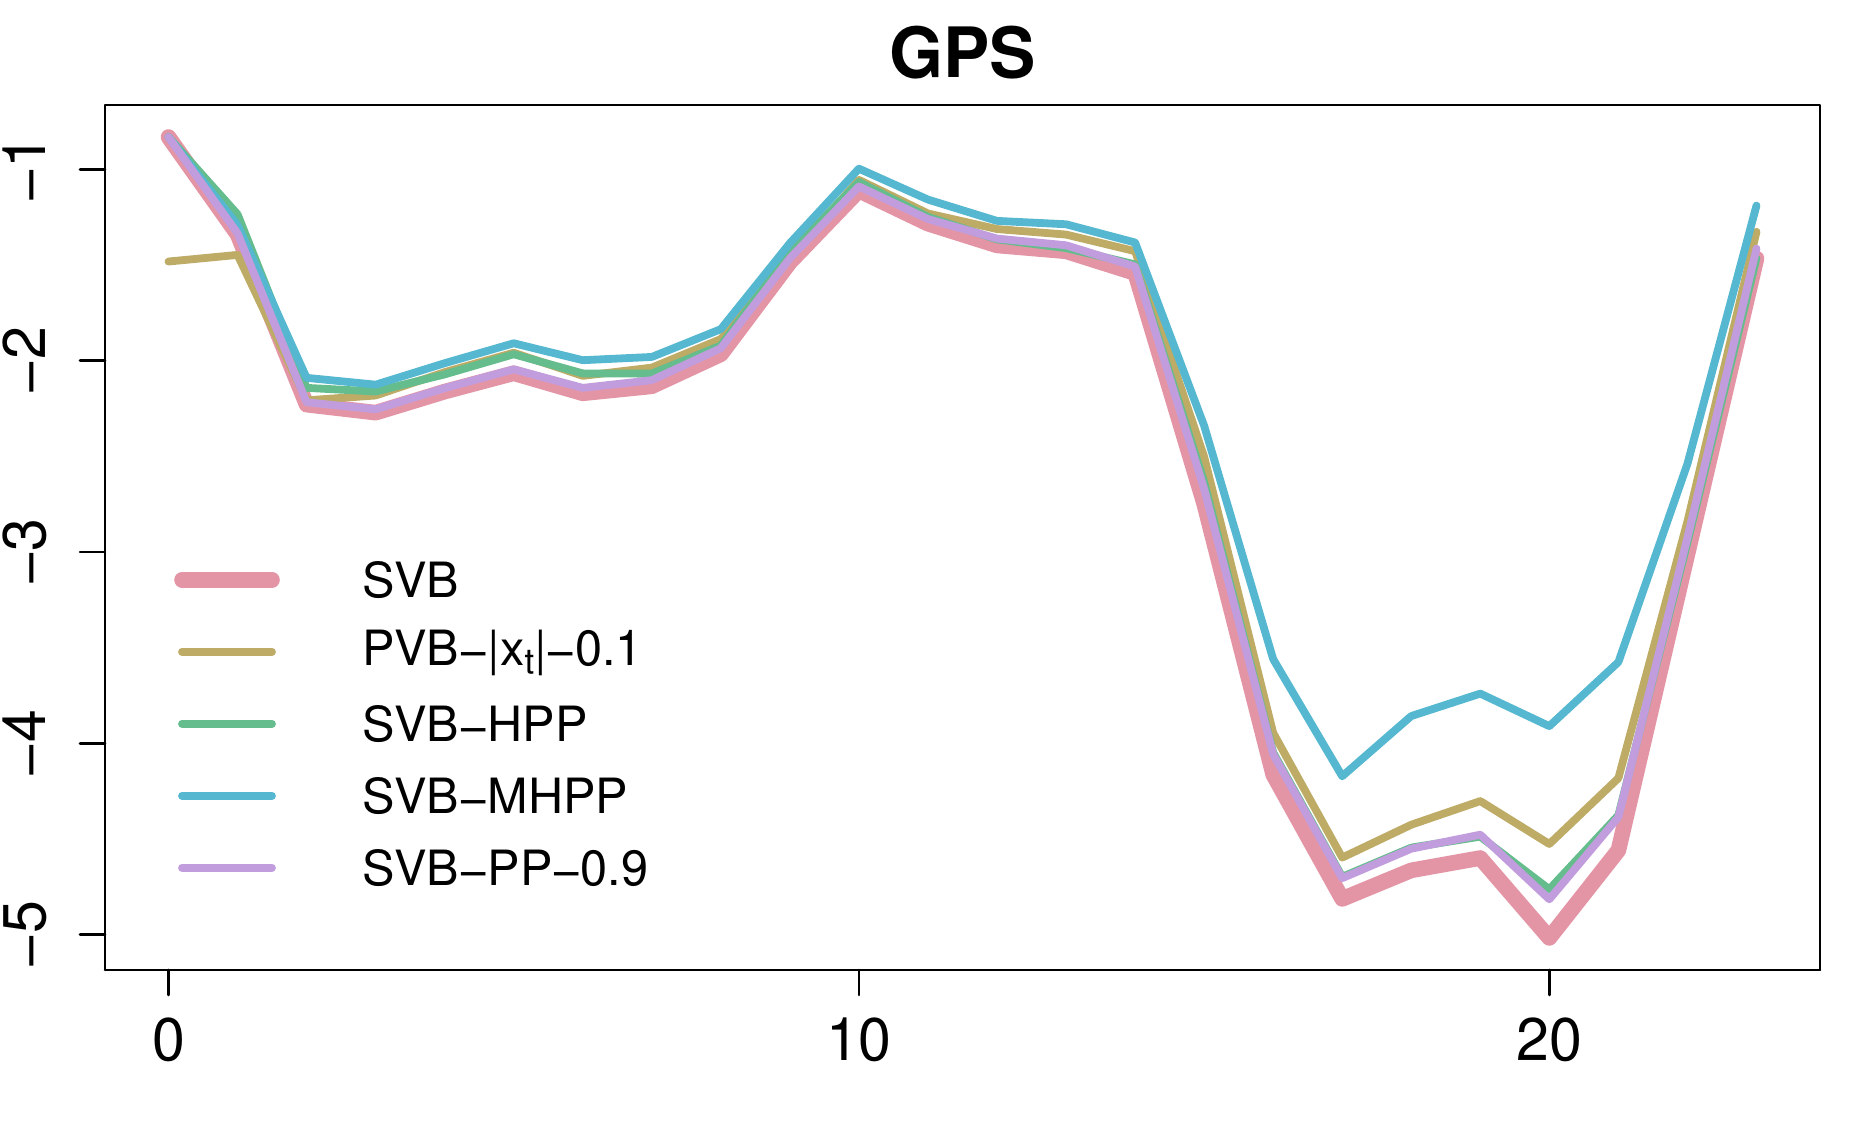}
%\begin{tabular}{cc}
%\includegraphics[scale=0.3]{figs/GPS-HOUR-TestMLL}&
%%\includegraphics[scale=0.2]{figs/GPS-HOUR-TotalMLL}&
%\includegraphics[scale=0.3]{figs/GPS-HOUR-RHO}\\
%(a) $TMLL_t$ & (b) $E[\rho_t]$ \\
%\end{tabular}
\caption{GPS}
\label{app:fig:exp:gps}
\end{center}
\vskip -0.2in
\end{figure*} 

\begin{figure*}[htb!]
\vskip 0.2in
\begin{center}
\includegraphics[width=8cm,height=4.5cm,keepaspectratio]{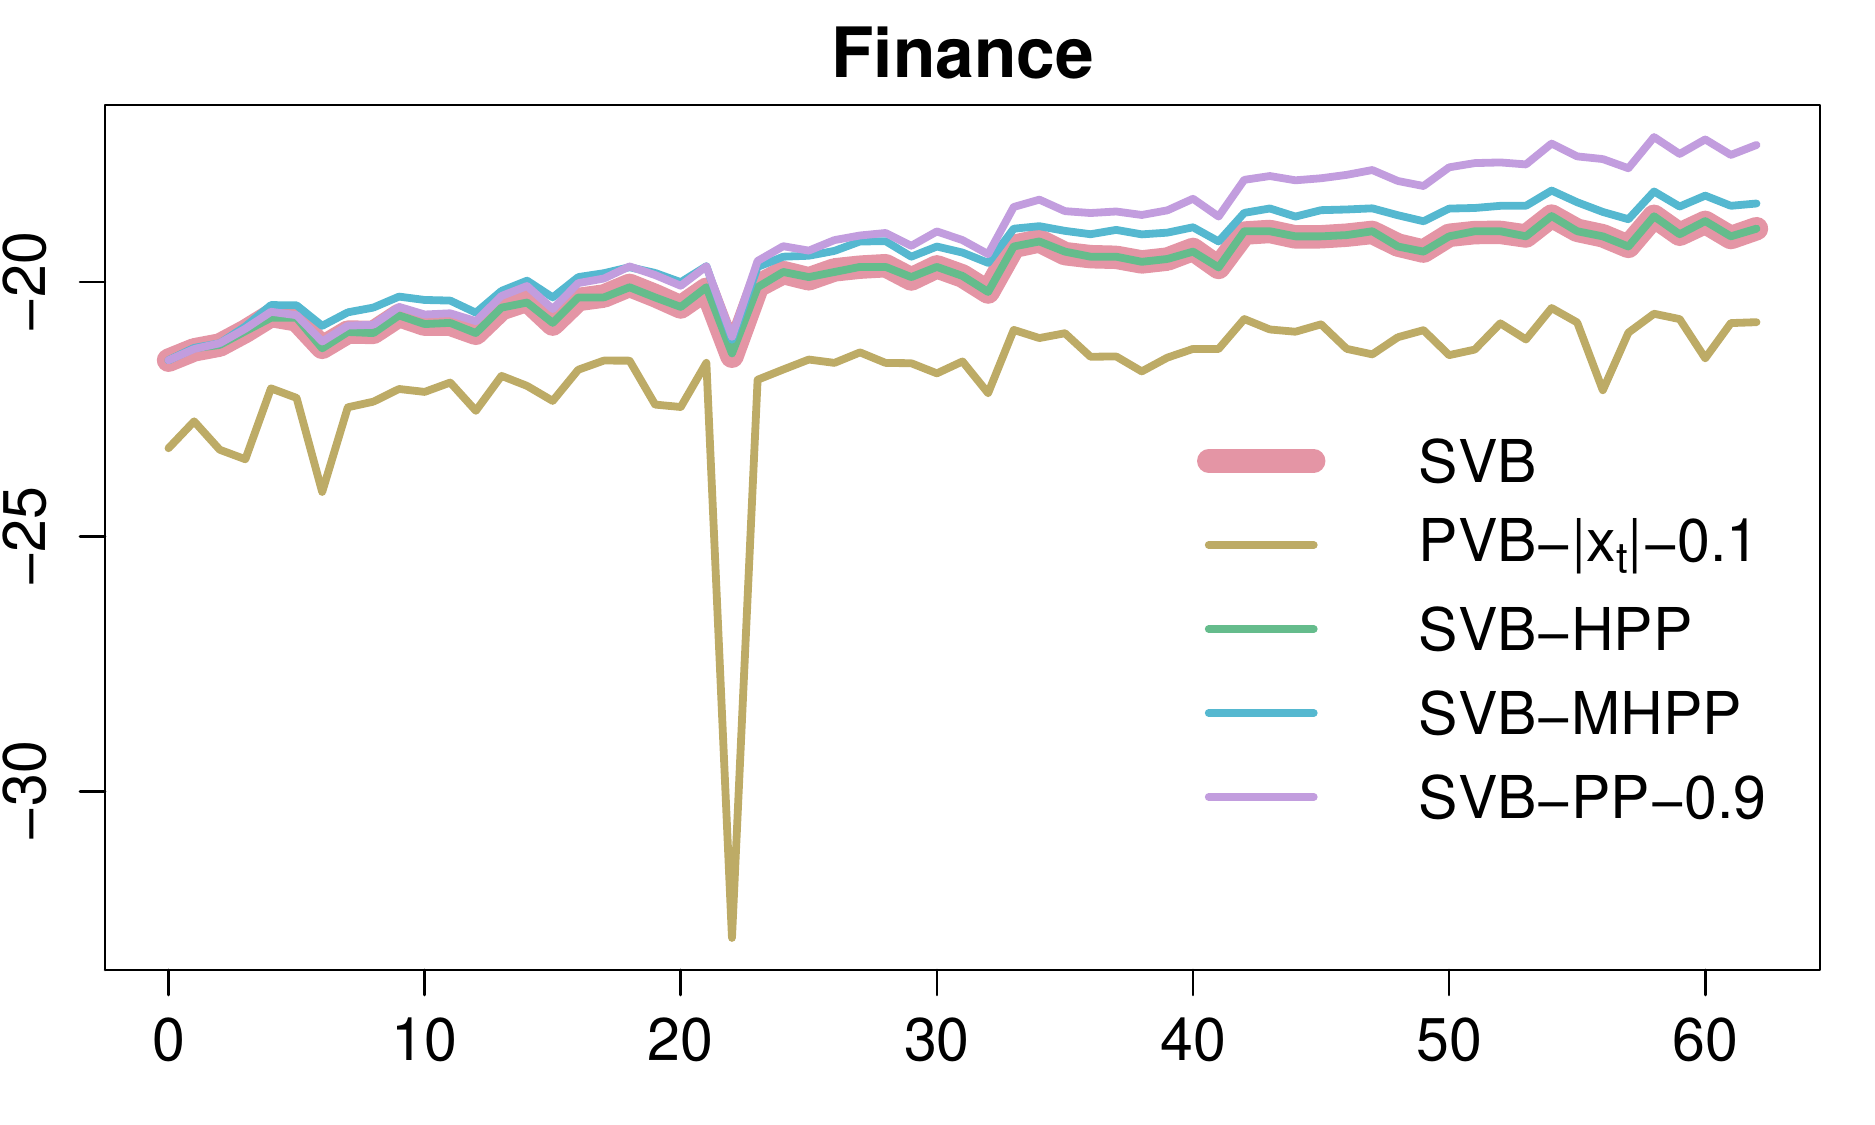}
%\begin{tabular}{cc}
%\includegraphics[scale=0.3]{figs/BCC-TestMLL}&
%%\includegraphics[scale=0.2]{figs/BCC-TotalMLL}&
%\includegraphics[scale=0.3]{figs/BCC-RHO}\\
%(a) $TMLL_t$ & (b) $E[\rho_t]$ \\
%\end{tabular}
\caption{BCC}
\label{app:fig:exp:bcc}
\end{center}
\vskip -0.2in
\end{figure*}
